# Supplementary material for: GraVITON: Graph based garment warping with attention guided inversion for Virtual-tryon
Source: arXiv:2406.02184 source file (2024-06-04)
Supplement: Supplementary file 1 [file supple_fig1.tex]

\centering
\begin{tabular}{c c c c c c} 
Garment & & &  & &  \\
        \includegraphics[width=0.25\linewidth, height=32mm]
        {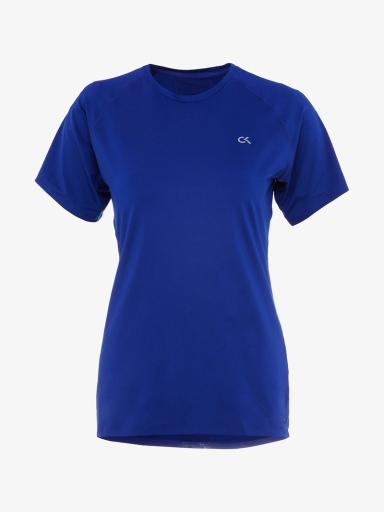} &
        \includegraphics[width=0.25\linewidth, height=32mm]
        {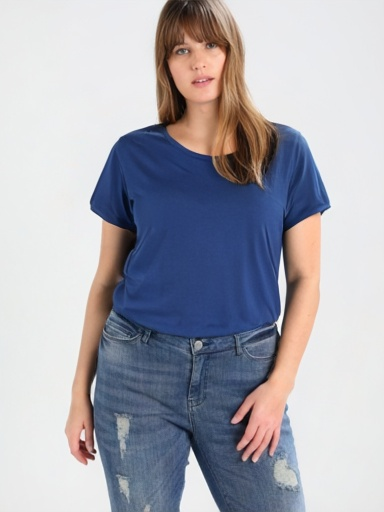} &
        \includegraphics[width=0.25\linewidth, height=32mm]{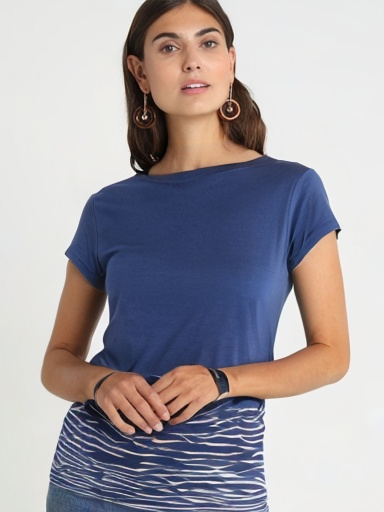} &
        \includegraphics[width=0.25\linewidth, height=32mm]{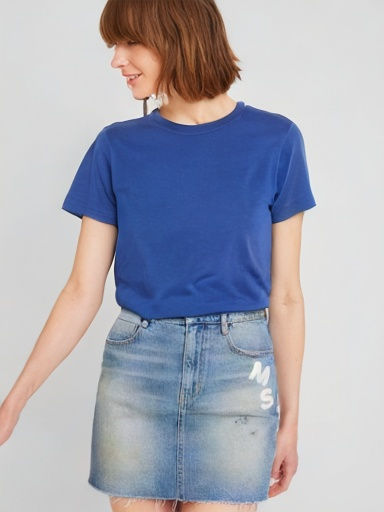} &
        \includegraphics[width=0.25\linewidth, height=32mm]{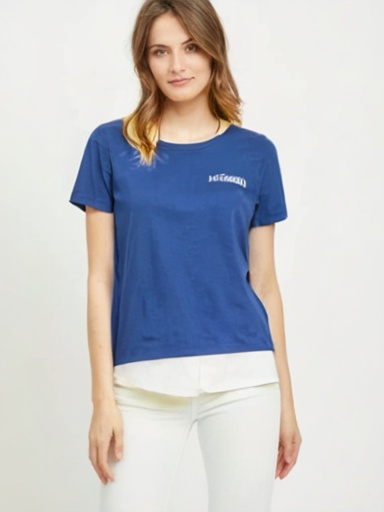}
          \\
        \includegraphics[width=0.25\linewidth, height=32mm]
        {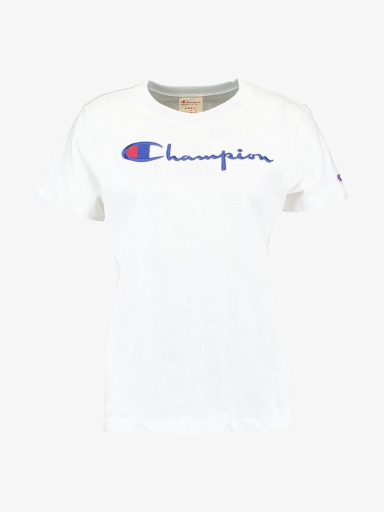} &
        \includegraphics[width=0.25\linewidth, height=32mm]
        {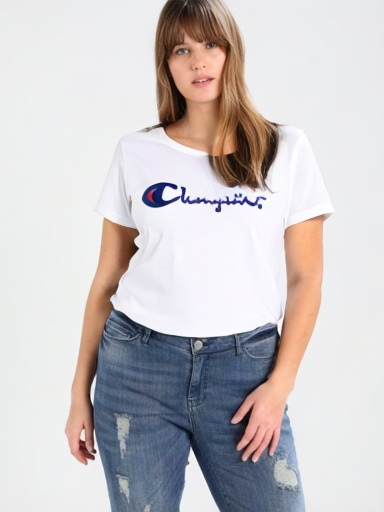} &
        \includegraphics[width=0.25\linewidth, height=32mm]{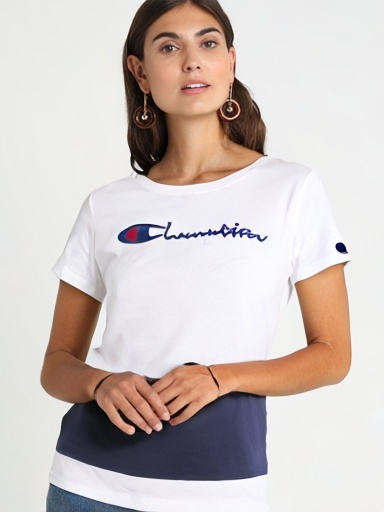} &
        \includegraphics[width=0.25\linewidth, height=32mm]{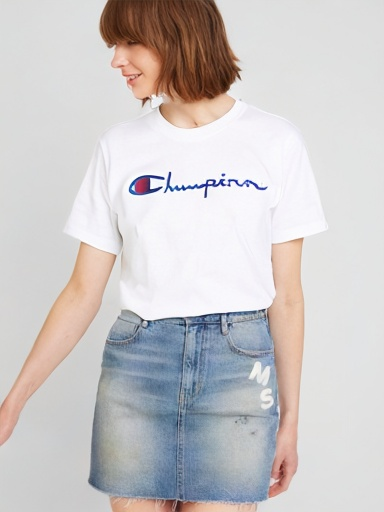} &
        \includegraphics[width=0.25\linewidth, height=32mm]{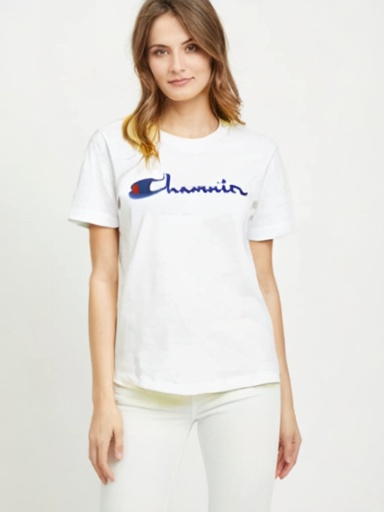}
         \\
        %   \includegraphics[width=0.25\linewidth, height=32mm]
        % {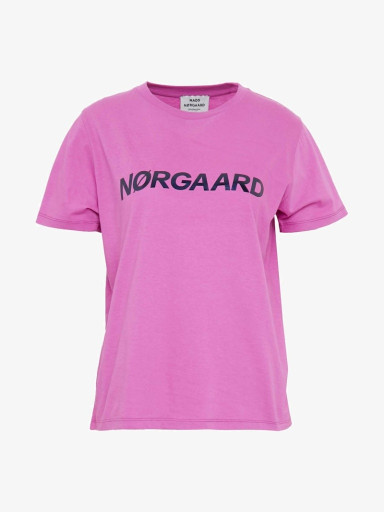} &
        % \includegraphics[width=0.25\linewidth, height=32mm]
        % {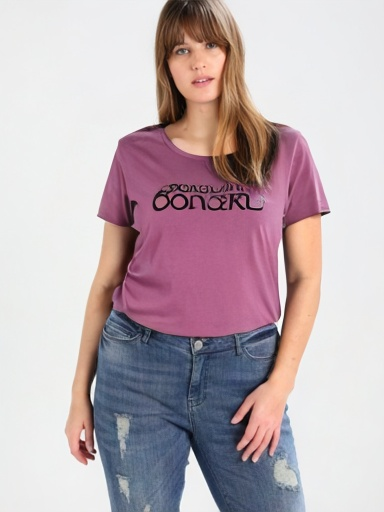} &
        % \includegraphics[width=0.25\linewidth, height=32mm]{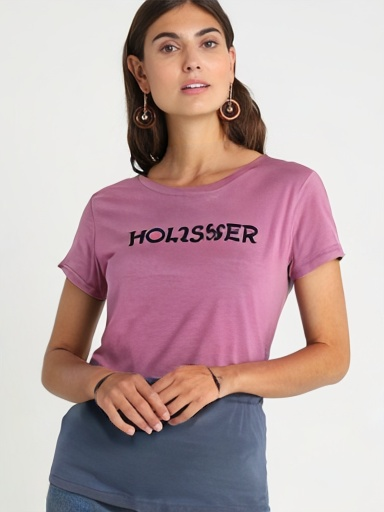} &
        % % \includegraphics[width=0.25\linewidth, height=32mm]{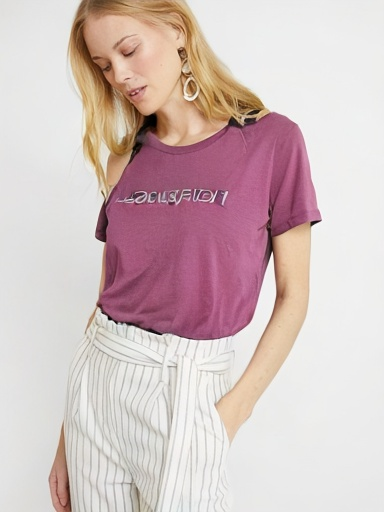} &
        % \includegraphics[width=0.25\linewidth, height=32mm]{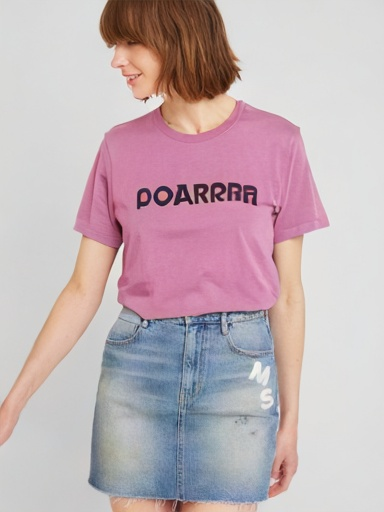} &
        % \includegraphics[width=0.25\linewidth, height=32mm]{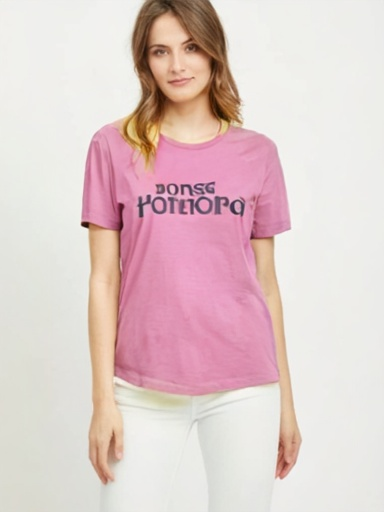}
        %  \\
          \includegraphics[width=0.25\linewidth, height=32mm]
        {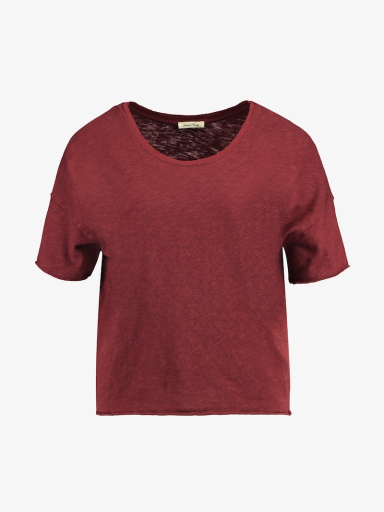} &
        \includegraphics[width=0.25\linewidth, height=32mm]
        {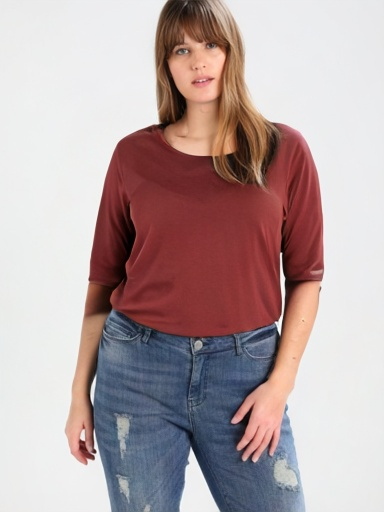} &
        \includegraphics[width=0.25\linewidth, height=32mm]{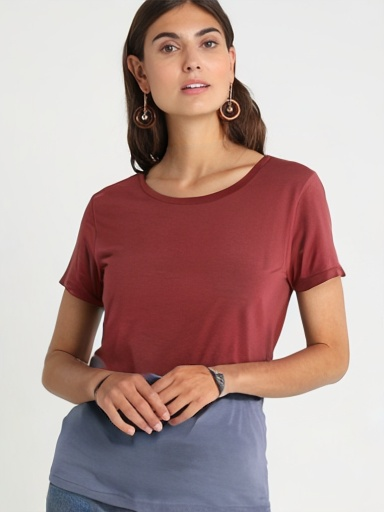} &
        \includegraphics[width=0.25\linewidth, height=32mm]{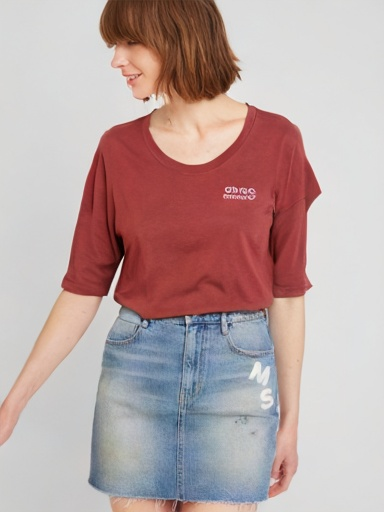} &
        \includegraphics[width=0.25\linewidth, height=32mm]{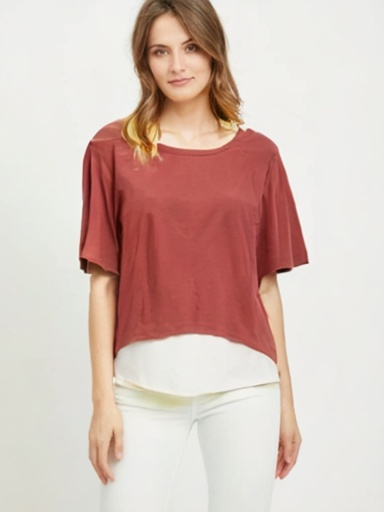}
         \\
    \end{tabular}
